# Supplementary material for: Open-Ended Visual Question-Answering
Source: arXiv:1610.02692 source file (2016-10-09)
Supplement: Supplementary file 1 [file automatic-question-answer-generation.pdf]

# Towards Automatic Generation of Question Answer Pairs from Images

Issey Masuda Mora, Santiago Pascual de la Puente, Xavier Giro-i-Nieto
Universitat Politecnica de Catalunya (UPC)
Barcelona, Catalonia/Spain
issey.masuda@alu-etsetb.upc.edu, santiago.pascual@tsc.upc.edu, xavier.giro@upc.edu

## Abstract

*This extended abstract presents our research in the generic field of Visual Question-Answering (VQA) focusing on a new branch that aims to generate question-answer pairs based on an image. To do so, we use the VQA dataset provided for the VQA challenge to train a Deep Neural Network which has the image as an input and two different outputs, the question and its associated answer.*

## 1. Introduction

Recurrent Neural Networks (RNNs) are widely used in many Natural Language Processing (NLP) tasks nowadays (e.g. language modelling, machine translation) for their good capacity to model sequences while Convolutional Neural Networks (CNNs) are more often used to process images in Computer Vision. Here we explore a model that joins both visual and textual features using Long Short-Term Memory networks (LSTM), a RNN extension, and an off-the-shelf model for visual features extraction in order to generate image-related Question-Answer Pairs (QAP).

## 2. Related Work

Different network architectures have been presented to solve Visual Question-Answering tasks [1, 2, 5, 6]. As a common approach, they all extract visual features from an image using CNNs, which have been proven to achieve state-of-the-art performance in image classification tasks. These visual features are combined with a vectorized representation of the question. The method to vectorize the question ranges from a simple Bag-Of-Words (BOW) representation [5] to the use of RNNs [2] to obtain an embedding of the question.

As for the generation of QAP, only a text-based study has been found. Serban *et al.* [3] propose an encoder-decoder architecture using GRU RNNs to generate a question from a fact, which is a tuple of subject, relationship, object. The model is trained in such a way that the answer to the generated question is the object from the fact.

## 3. Model

Figure 1 depicts our model architecture that is discussed below.

**Visual features extraction.** We consider using the model VGG-16 net [4] to extract the visual features from the input image. These features are not the output of the final softmax layer of the net but the output of the last max-pooling (before the fc-4096 layer).

**Question generation.** The visual features are injected into a Long Short-Term Memory (LSTM) RNN that will learn how to generate an embedding of the question. This embedding will then be fed into a softmax layer of dimension equal to our vocabulary size, which in turn will predict the n-th word of the question. At each time-step, the same visual features are shown to the model, which will produce one question word at a time. The maximum question length is then a parameter to specify to the model, but the question can have less words if an End of Sentence (EOS) is predicted. Notice that at the output of the LSTM we will have an embedding of the question word being predicted.

**Answer prediction.** The question embedding will then be given to another LSTM in charge of producing the answer to the question. This module also receives the visual features of the image extracted with the VGG-16 as an input. Only the last state of this LSTM will be used to predict the answer, as only at that moment the network will have seen all the question. Again, a softmax layer will be used to obtain the predicted word.

**Training** We train the model end-to-end (E2E) freezing the VGG-16 layer weights. The dataset used to train the model is the one provided for the Visual Question Answering challenge[1], which provides three questions per image and ten answers per question.

[1] http://www.visualqa.org/

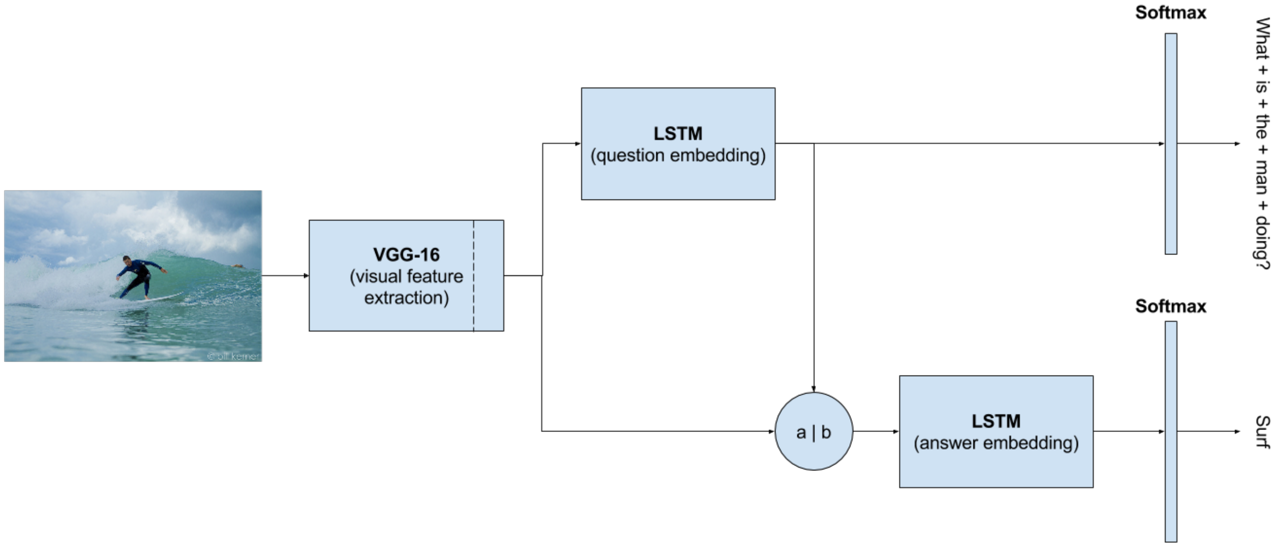


Figure 1. Automatic QA generation model. LSTMs are used to generate sequences of words

# 4. Applications

A model able to generate question-answer pairs present a wide number of different interesting applications:

- **Synthetic dataset generation:** Similarly to [3], a corpus of Visual-Question-Answer tuples can be generated using this approach to increase existing datasets such as VQA dataset. With a technique able to produce more examples for visual question-answering tasks, we can offer to the research community a broader dataset to train their models with. Given the nature of this dataset, it could be use to train the models but not for testing purposes.

- **Pedagogy applications for kids:** Building a model that can ask questions related to images to the kids (such as 'What is on the table?') can be a very effective tool to help them learn the language in an interactive way and more important, in a customize way. Using own images could ease the process of linking together objects/spaces with their names.

- **Language learning:** With the same spirit than the previous example, applications to help users to learn a new language can be very appealing.

# 5. Conclusions

We have proposed a model that can generate QAPs given an image. We use an off-the-shelf model to extract the visual features from the image and two RNN blocks to predict the question and answer. We also expose some of the applications where such a model could be used to.

# References


[1] S. Antol, A. Agrawal, J. Lu, M. Mitchell, D. Batra, C. Lawrence Zitnick, and D. Parikh. Vqa: Visual question answering. In *Proceedings of the IEEE International Conference on Computer Vision*, pages 2425–2433, 2015.

[2] H. Noh, P. H. Seo, and B. Han. Image question answering using convolutional neural network with dynamic parameter prediction. In *IEEE conference on Computer Vision and Pattern Recognition*, 2016.

[3] I. V. Serban, A. García-Durán, C. Gulcehre, S. Ahn, S. Chandar, A. Courville, and Y. Bengio. Generating factoid questions with recurrent neural networks: The 30m factoid question-answer corpus. *arXiv preprint arXiv:1603.06807*, 2016.

[4] K. Simonyan and A. Zisserman. Very deep convolutional networks for large-scale image recognition. In *International Conference on Learning Representations*, 2015.

[5] B. Zhou, Y. Tian, S. Sukhbaatar, A. Szlam, and R. Fergus. Simple baseline for visual question answering. *arXiv preprint arXiv:1512.02167*, 2015.

[6] Y. Zhu, O. Groth, M. Bernstein, and L. Fei-Fei. Visual7w: Grounded question answering in images. In *IEEE conference on Computer Vision and Pattern Recognition*, 2016.
